# Supplementary material for: Detection of Technical Debt in Java Source Code
Source: arXiv:2411.05457 source file (2025-08-09)
Supplement: Supplementary file 1 [file Appendix.tex]

\appendices

\section{RQ3}\label{sec:appedix_rq3}

\begin{tcolorbox}[colback=blue!5!white,colframe=gray!50!black,title=Input template for Decoder-based PTMs]
Task: Analyze the provided code the provided code to identify technical debts, which can be categorized into the following four types:\\

DESIGN: indicate misplaced code, lack of abstraction, long methods, poor implementation, workarounds or a temporary solution.

IMPLEMENTATION: incompleteness of the functionality in the method, class or program

DEFECT: bugs or errors in the code that affect functionality.

TEST: express the need for creation or improvement of the current set of tests.

If the code does not exhibit any of these types of technical debt, respond with NonTD.\\
 
Code to Analyze: \{code\}

Answer: 
\end{tcolorbox}

\begin{table*}[t]
\scriptsize
\centering
\caption{F1-score performance of 16 PLMs on TD detection using \TScode across 10 folds. \textbf{Bold scores} indicate the highest score, while \underline{Underlined scores} represent the second highest.}
\begin{adjustbox}{width=\textwidth}
\begin{tabular}{l|c|c|c|c|c|c|c|c|c|c|c}
\toprule
Model & 0 & 1 & 2 & 3 & 4 & 5 & 6 & 7 & 8 & 9\\
\midrule
CodeBERT & \textbf{50.51} & 34.09 & \underline{53.72} & \underline{48.12} & \textbf{45.16} & 48.35 & 34.90 & 41.21 & 45.06 & 33.58 \\
UniXCoder & 32.31 & \underline{41.85} & 51.13 & 46.26 & 38.65 & 55.28 & 41.38 & 39.43 & 44.95 & 34.56 \\
GraphCodeBERT & 41.50 & \textbf{43.18} & \textbf{55.18} & 43.48 & 34.77 & 55.10 & \textbf{44.31} & 43.18 & \underline{46.30} & 35.07 \\
RoBERTa & 43.54 & 30.68 & 41.42 & 38.26 & 39.78 & 42.42 & 32.16 & 46.36 & 36.73 & 30.85 \\
ALBERT & 42.75 & 33.33 & 48.48 & 44.66 & 39.22 & 52.63 & 37.33 & 42.06 & 42.90 & 36.51 \\
\midrule
PLBART & 31.27 & 34.43 & 45.95 & 40.80 & 39.36 & 53.93 & 33.72 & 38.20 & 41.90 & 39.42 \\
CodeT5 & 25.85 & 33.70 & 34.95 & 32.47 & 34.40 & 47.56 & 35.63 & 36.04 & 34.71 & 38.77 \\
CodeT5+ & 35.37 & 37.96 & 44.98 & 44.54 & 41.13 & \underline{55.56} & 38.31 & 45.35 & 42.20 & 34.20 \\
\midrule
TinyLlama & 42.18 & 34.10 & 43.37 & 41.09 & 43.01 & 50.27 & 32.56 & 37.88 & 41.98 & 34.09 \\
DeepSeek-Coder & 48.30 & 37.55 & 50.81 & 41.09 & \underline{44.44} & \textbf{60.88} & 40.31 & \underline{51.52} & \textbf{46.60} & \textbf{40.35} \\
OpenCodeInterpreter & \underline{50.34} & 30.27 & 47.25 & 39.66 & 34.05 & 52.62 & 39.53 & 45.45 & 42.59 & 35.84 \\
Phi-2 & 44.22 & 32.58 & 44.50 & \textbf{51.01} & 43.01 & 51.24 & 38.43 & 34.55 & 41.05 & 35.07 \\
Starcoder2 & 44.56 & 35.48 & 52.59 & 45.11 & 38.65 & 50.14 & \underline{42.15} & 35.40 & 38.84 & 34.81 \\
CodeLlama & 27.55 & 29.89 & 45.95 & 45.98 & 35.48 & 50.55 & 35.27 & 37.73 & 33.64 & \underline{39.60} \\
Magicoder & 32.65 & 33.72 & 45.31 & 41.38 & 41.22 & 52.89 & 41.47 & \textbf{54.24} & 41.67 & \textbf{40.35} \\

\bottomrule
\end{tabular}
\end{adjustbox}
\label{tab:RQ3_10folds}
\end{table*}

\section{RQ2}

\begin{figure*}
\centering
\begin{subfigure}[b]{0.48\textwidth}
 \centering
 \includegraphics[width=\textwidth]{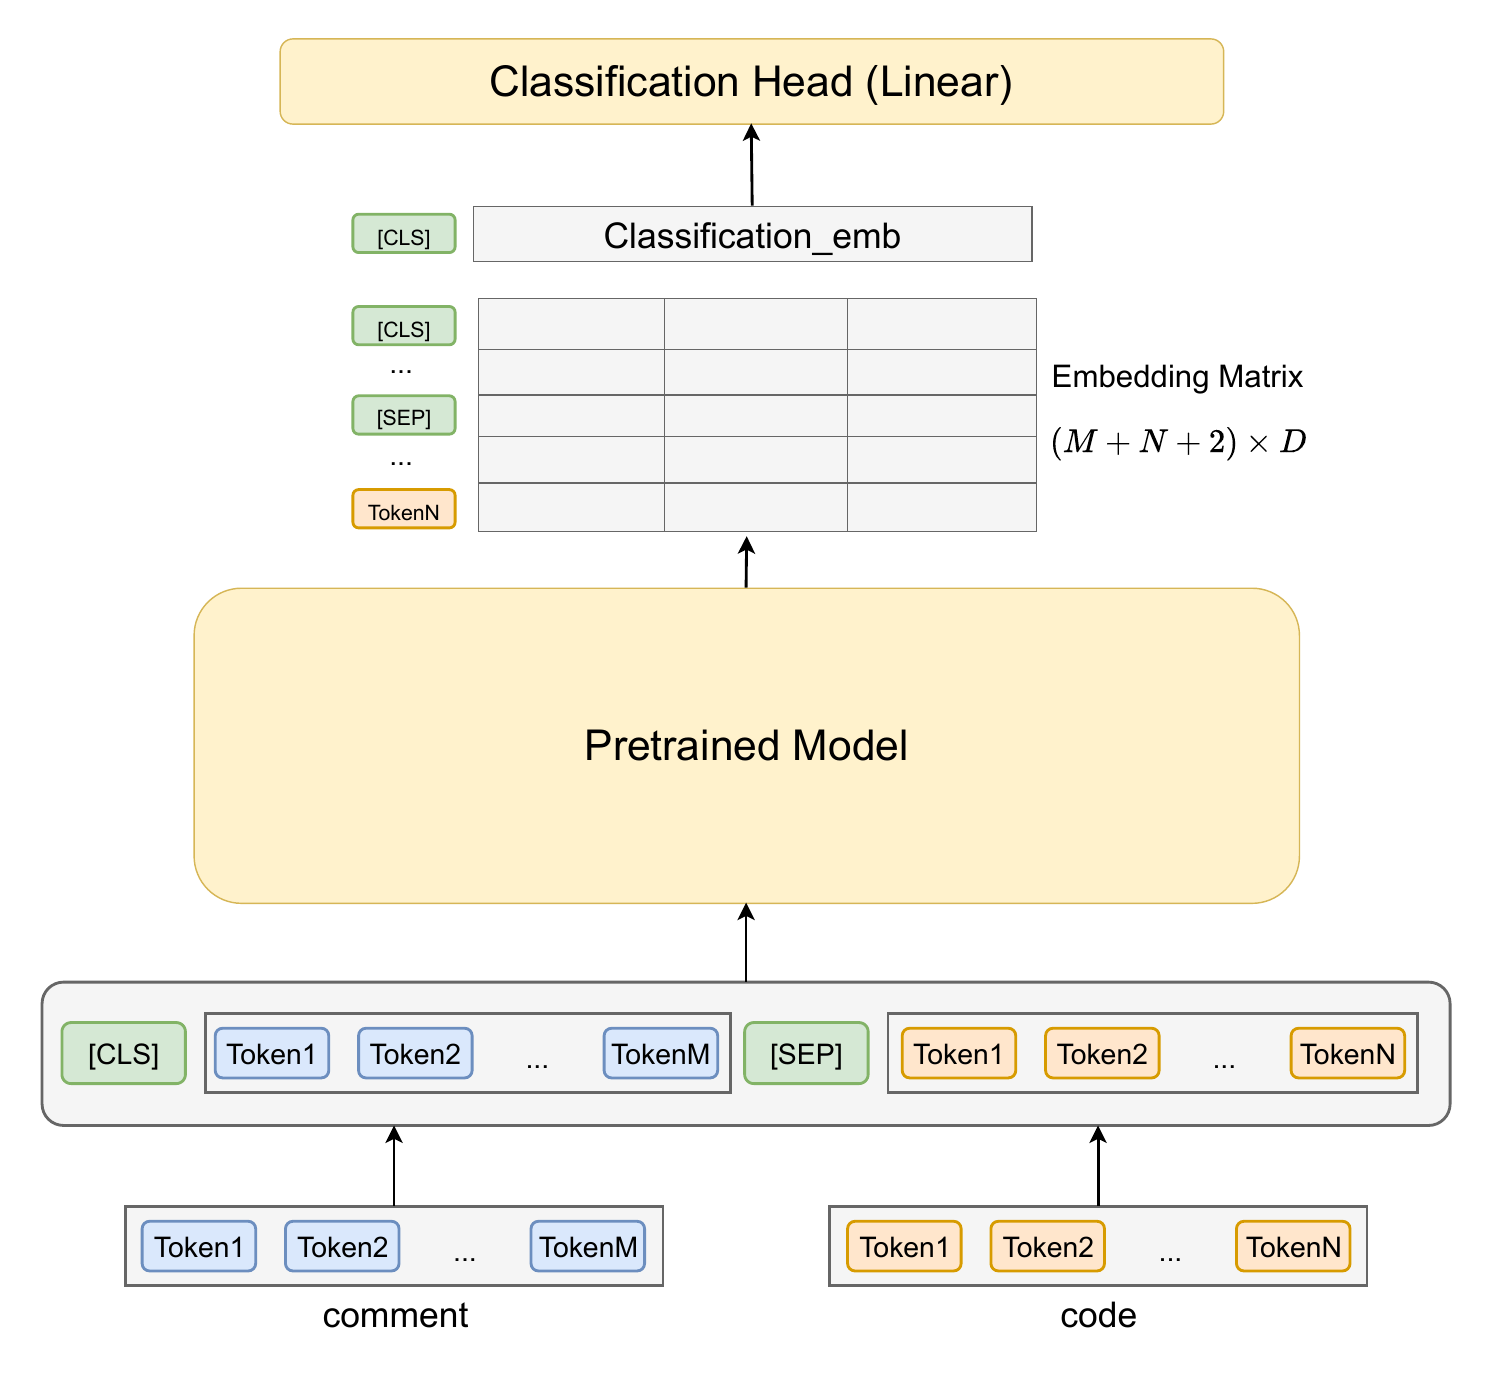}
 \caption{StrConcat}
\end{subfigure}
\hfill
\begin{subfigure}[b]{0.48\textwidth}
 \centering
 \includegraphics[width=\textwidth]{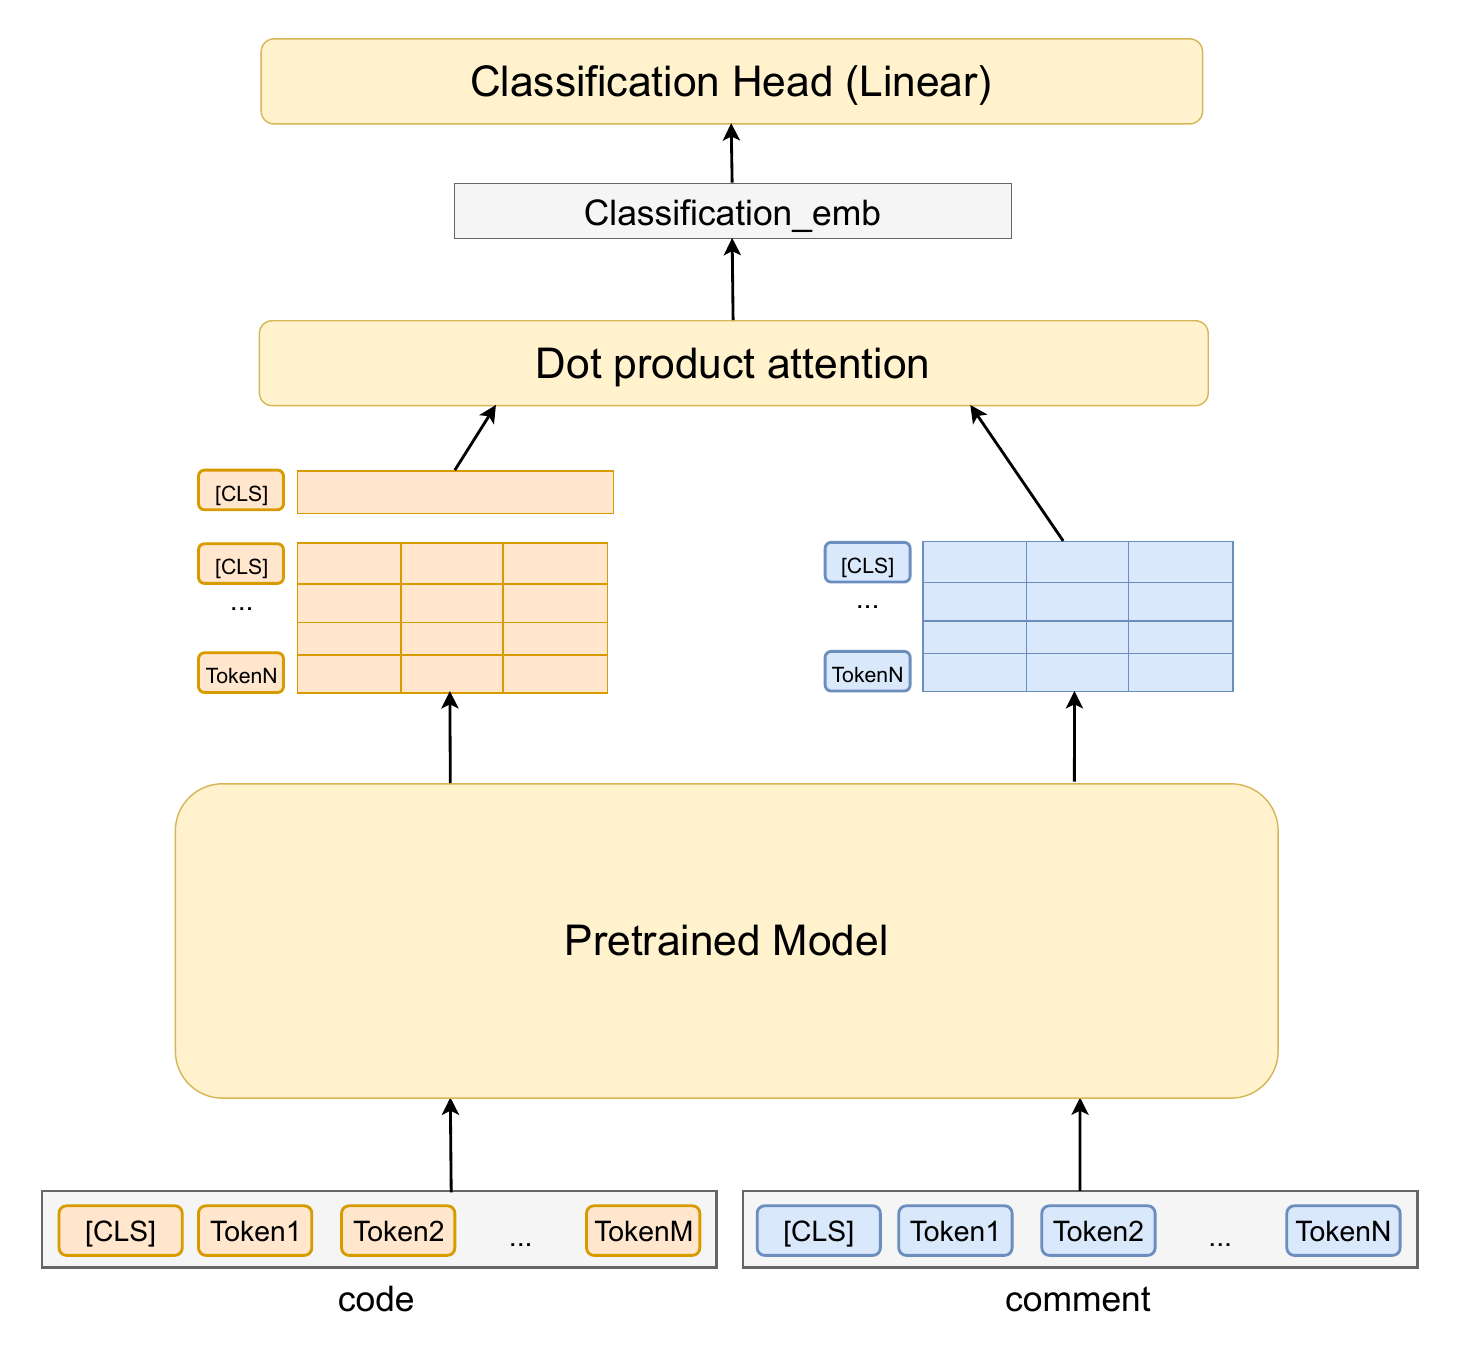}
 \caption{CodeAtt}
\end{subfigure}
\hfill
\caption{Integration techniques: StrConcat and CodeAtt.}
\label{fig:code_comment_concat}
\end{figure*}

\begin{figure}[t!]
\centering
\small
\includegraphics[width=0.48\textwidth]{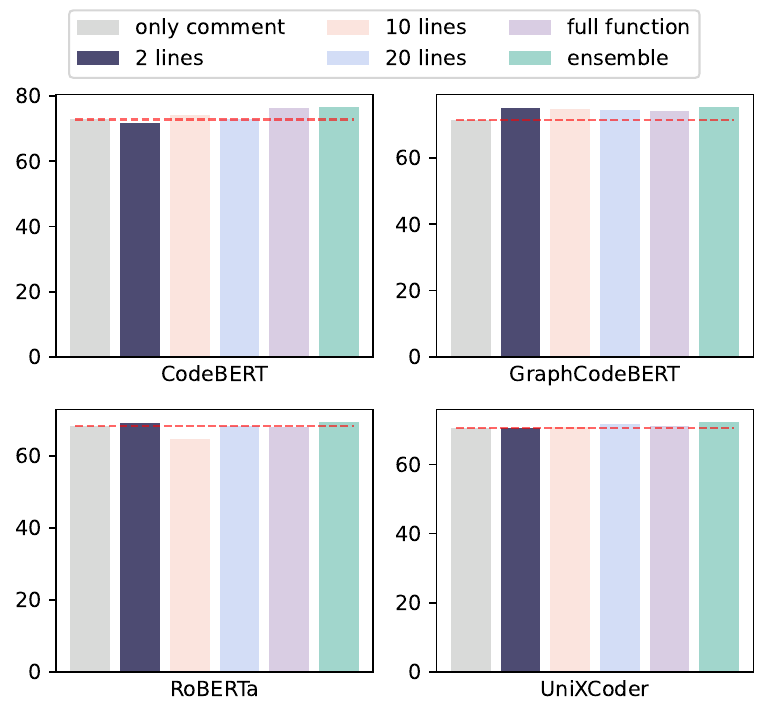}
\caption{F1-scores of four PLMs evaluated across different scopes of code context with StrConcat technique. The red dashed line ({\color{red} - -}) denotes the performance of models using only comment.}
\label{fig:strconcat_context}
\end{figure}

\newpage
\onecolumn
\begingroup
\begin{longtable}{|p{0.05\textwidth}|p{0.35\textwidth}|p{0.55\textwidth}|}
\hline
\textbf{Debt} & \textbf{Comment} & \textbf{Source code}\\ 
\hline \hline
\multirow{50}{*}{\rotatebox{90}{\textbf{\textit{design}}}}
&
\begin{minted}[breaklines]{java}
// TODO: check here, may be necessary to remove the last space.
\end{minted}

&
\begin{minted}[breaklines]{java}
private void generateArttribute() {
    String temp = "";
    for (String s : connectedElements)
        temp = temp + s + " ";
        // TODO: check here, may be necessary to remove the last space.
        linkingResourceElement.setAttribute(
        "connectedResourceContainers_LinkingResource", temp);
}
\end{minted} 
\\\cline{2-3}
&
\begin{minted}[breaklines]{java}
// TODO: Configuration is not used because we don't support any other mode for now. For that : ISPN-8413
\end{minted}
&
\begin{minted}[breaklines]{java}
@Override
public boolean defineLock(String name, ClusteredLockConfiguration configuration) {
  // TODO: Configuration is not used because we don't support any other mode for now. For that : ISPN-8413
  CacheHolder cacheHolder = extractCacheHolder(cacheHolderFuture);
  cache = cacheHolder.getClusteredLockCache();
  ClusteredLockKey key = new ClusteredLockKey(ByteString.fromString(name));
  ClusteredLockValue clusteredLockValue = cache.putIfAbsent(key, ClusteredLockValue.INITIAL_STATE);
  locks.putIfAbsent(name, new ClusteredLockImpl(name, key, cache, this));
  return clusteredLockValue == null;
}
\end{minted} 
\\\cline{2-3}
&
\begin{minted}[breaklines]{java}
// TODO, assume the url is a file path for now.
\end{minted}
&
\begin{minted}[breaklines]{java}
@GET
@Path("getDefaultNotebook")
@Produces(MediaType.TEXT_PLAIN)
public String getDefaultNotebook() {
    final String defaultNotebookUrl = this.bkConfig.getDefaultNotebookUrl();
    // TODO, assume the url is a file path for now.
    java.nio.file.Path defaultNotebookFile = Paths.get(defaultNotebookUrl);
    String content = this.utils.readFile(defaultNotebookFile);
    if (content == null) {
      System.out.println("Warning, default notebook is empty");
      return "";
    }
    return clean(content);
}
\end{minted}
\\\cline{2-3}
&
\begin{minted}[breaklines]{java}
// This cast is horrid but we can't fix everything at once.
\end{minted}
&
\begin{minted}[breaklines]{java}
void tracksDropped(Point startPoint, Point dropPoint, List<Track> tracks) {
    // This cast is horrid but we can't fix everything at once.
    TrackPanel panel = ((TrackPanel) getParent());
    List<MouseableRegion> regions = getMouseRegions();
    if (regions.isEmpty()) {
        // empty panel,  just add the tracks
        panel.addTracks(tracks);
    } else {
    ...
}
\end{minted}
\\\midrule

\multirow{50}{*}{\rotatebox{90}{\textbf{\textit{implementation}}}} &
\begin{minted}[breaklines]{java}
//TODO Find a way to re-send the message.
\end{minted}
&
\begin{minted}[breaklines]{java}
public static void addChatMessageFixed(ICommandSender sender, IChatComponent message) {
    if (sender == null || message == null) return;
    if (sender instanceof EntityPlayerMP) {
        if (((EntityPlayerMP)sender) .playerNetServerHandler != null) {
            sender.addChatMessage(message);
        } else {
            //TODO Find a way to re-send the message.
        }
    } else {
        sender.addChatMessage(message);
    }
}
\end{minted}
\\\cline{2-3}
&
\begin{minted}[breaklines]{java}
// TODO: More checking here - actually parse out tile coord
\end{minted}
&
\begin{minted}[breaklines]{java}
@Override
public boolean accept(File pathname)
{
    // TODO: More checking here - actually parse out tile coord
    return pathname.isFile() && pathname.getName().endsWith(".tile");
}
\end{minted}
\\\cline{2-3}
&
\begin{minted}[breaklines]{java}
// TODO show resulting document
\end{minted}
&
\begin{minted}[breaklines]{java}
public static final int testElementParsing (
    final PrintStream out, final BufferedReader in, final String ... args)
{
    final String ans=getval(out, in, "use owner document y/[n]/q");
    ...
    
    final int nErr=testElementParsing(out, in, owner, args);
        if (owner != null)
        {
            // TODO show resulting document
        }
        return nErr;
}
\end{minted}
\\\cline{2-3}
&
\begin{minted}[breaklines]{java}
// TODO This will be implemented in the next version
\end{minted}
&
\begin{minted}[breaklines]{java}
@Override
public int write(ChannelBuffer cb) {
    // TODO This will be implemented in the next version
    return 0;
}
\end{minted} 
\\\midrule
\multirow{50}{*}{\rotatebox{90}{\textbf{\textit{defect}}}}
&
\begin{minted}[breaklines]{java}
//Do not use getClass() here... a typical weld issue...
\end{minted}
&
\begin{minted}[breaklines]{java}
@PostConstruct
public void setup(){
    //Do not use getClass() here... a typical weld issue...
    endpointUrl=appConfiguration.getBaseEndpoint() + ServiceProviderConfigWS.class.getAnnotation (Path.class).value();
}
\end{minted} 
\\\cline{2-3}
&
\begin{minted}[breaklines]{java}
// the following stuff did not work and I don't know why!
\end{minted}
&
\begin{minted}[breaklines]{java}
private void detectTitle() {
    Document doc = this.contentView.getDocument();
    if (doc instanceof HTMLDocument) {
      HTMLDocument hdoc = (HTMLDocument)doc;
      System.out.println("Document Property:" + hdoc.getProperty(Document.TitleProperty));
      // the following stuff did not work and I don't know why!
      Element element = hdoc.getElement(hdoc.getDefaultRootElement(), StyleConstants.NameAttribute, HTML.Tag.TITLE);
      if (element != null && element.getStartOffset() >= 0) {
      ...
}
\end{minted} 
\\\cline{2-3}
&
\begin{minted}[breaklines]{java}
/* POTENTIAL FLAW: Use password directly in PasswordAuthentication() */
\end{minted}
&
\begin{minted}[breaklines]{java}
public void bad() throws Throwable
{
    String password = (new CWE319_Cleartext_Tx_Sensitive_Info __URLConnection_passwordAuth_61b()).badSource();
    if (password != null)
    {
        /* POTENTIAL FLAW: Use password directly in PasswordAuthentication() */
        PasswordAuthentication credentials = new PasswordAuthentication("user", password.toCharArray());
        IO.writeLine(credentials.toString());
    }
}
\end{minted}
\\\cline{2-3}
&
\begin{minted}[breaklines]{java}
// FIXME: These record counts are only correct iff if duplicate keys are disregarted.
// This is unfortunate. Keys are currently only considered based their SKSKode.
// They should be a combination of type + kode + startdato based on the register doc.
\end{minted}
&
\begin{minted}[breaklines]{java}
@Test
public void canImportTheCorrectNumberOfRecords() throws Throwable {
    process(shakParser, shakDao, "data/sks/SHAKCOMPLETE.TXT");
    // FIXME: These record counts are only correct iff if duplicate keys are disregarted.
    // This is unfortunate. Keys are currently only considered based their SKSKode.
    // They should be a combination of type + kode + startdato based on the register doc.
    assertEquals(1017, jdbc.queryForInt("SELECT COUNT(*) FROM class_shak WHERE Organisationstype = 'Sygehus'"));
    assertEquals(18411, jdbc.queryForInt("SELECT COUNT(*) FROM class_shak WHERE Organisationstype = 'Afdeling'"));
    process(sksParser, sksDao, "data/sks/SKScomplete.txt");
    ...
}

\end{minted}
\\\midrule
\multirow{50}{*}{\rotatebox{90}{\textbf{\textit{documentation}}}}
&
\begin{minted}[breaklines]{java}
/** GETTER
 * TODO: Write general description for this method
 */
\end{minted}
&
\begin{minted}[breaklines]{java}
/** GETTER
 * TODO: Write general description for this method
 */
@JsonGetter("amount")
public int getAmount ( ) { 
    return this.amount;
}

\end{minted}
\\\cline{2-3}
&
\begin{minted}[breaklines]{java}
// TODO: document me
\end{minted}
&
\begin{minted}[breaklines]{java}
public void setCl(boolean b) {
    // TODO: document me
    this.tr.setResolveContLines(b);
}

\end{minted}
\\\cline{2-3}
&
\begin{minted}[breaklines]{java}
// TODO(saurabh): Explain reload scenario here
\end{minted}
&
\begin{minted}[breaklines]{java}
public void removeSegment(IndexSegment segment) {
    // TODO(saurabh): Explain reload scenario here
    Iterator<PrimaryKey> primaryKeyIterator = getPrimaryKeyIterator(segment, _primaryKeyColumns);
    while (primaryKeyIterator.hasNext()) {
      PrimaryKey pk = primaryKeyIterator.next();
      ...
}

\end{minted}
\\\cline{2-3}
&
\begin{minted}[breaklines]{java}
/**
 * A Factory Method pattern which creates an empty a BackedList
 * implementation
 * 
 * @return DOCUMENT ME!
 */
\end{minted}
&
\begin{minted}[breaklines]{java}
/**
 * A Factory Method pattern which creates an empty a BackedList
 * implementation
 * 
 * @return DOCUMENT ME!
 */
protected List createEmptyList() {
    return new BackedList(this, contentList(), 0);
}

\end{minted}
\\\midrule
\multirow{50}{*}{\rotatebox{90}{\textbf{\textit{testing}}}}
&
\begin{minted}[breaklines]{java}
//This unit-test class is the wrong place to test that behaviour, unless it becomes an integration test
//Given
\end{minted}
&
\begin{minted}[breaklines]{java}
@Test
public void simpleEndpointReturnsPostsWithoutTransformation() {
    //This unit-test class is the wrong place to test that behaviour, unless it becomes an integration test
    //Given
    ForumPosts posts = generateTestPosts();
    when(exampleApiService.getPosts()) .thenReturn(posts);
    //When
    ForumPosts controllerOutput = exerciseController.posts();
    //Then
    assertEquals(controllerOutput.size(), 2);
    assertTrue(controllerOutput.get(0).getTitle() .contains("Test"));
}
\end{minted}
\\\cline{2-3}

&
\begin{minted}[breaklines]{java}
// TODO(lwhite): Better tests
\end{minted}
&
\begin{minted}[breaklines]{java}
@Test
public void testReadFailure() throws IOException {
    // TODO (lwhite): These tests don't fail. What was their intent?
    Table table1 = Table.read()
            .csv(CsvReadOptions.builder( "../data/read_failure_test.csv") .minimizeColumnSizes());
    table1.structure(); // just make sure the import completed
    ShortColumn test = table1.shortColumn("Test");
    // TODO(lwhite): Better tests
    assertNotNull(test.summary());
}
\end{minted}
\\\cline{2-3}

&
\begin{minted}[breaklines]{java}
// TODO: Expand coverage
\end{minted}
&
\begin{minted}[breaklines]{java}
@Test
public void testAddressCreateAsBtcOnTestnet() {
    Network network = Network.findBuiltin("bitcoin-testnet").get();
    Optional<Address> ob1 = Address. create("mm7DDqVkFd35XcWecFipfTYM5dByBzn7nq", network);
    assertTrue(ob1.isPresent());
    Address b1 = ob1.get();
    assertEquals("mm7DDqVkFd35XcWecFipfTYM5dByBzn7nq", b1.toString());
    // TODO: Expand coverage
}
\end{minted}
\\\cline{2-3}

&
\begin{minted}[breaklines]{java}
/**
 *
 * TODO figure out how to test this
 *
 * @throws Exception
 */
\end{minted}
&
\begin{minted}[breaklines]{java}
/**
 *
 * TODO figure out how to test this
 *
 * @throws Exception
 */
public void testEmit() throws Exception {
    eh.on("ok", new EventEmitter.Listener() {
        @Override
        public void onEvent(Object data) {
            String ss = (String) data;
            if (ss == "ok")
                Log.d(TAG, "pass@" + ss);
            else
                Log.d(TAG, "fail@" + ss);
        }
    });
    ...
}
\end{minted}
\\\bottomrule
\caption{Examples of comments and corresponding source code for each type of SATD}
\label{tab:examples_data}
\end{longtable}

\endgroup
